# Supplementary material for: Seed-Point Detection of Clumped Convex Objects by Short-Range Attractive Long-Range Repulsive Particle Clustering
Source: arXiv:1804.04071 ancillary file (2018-04-11)
Supplement: Supplementary file 1 [file supplemental_notes_and_figures.pdf]

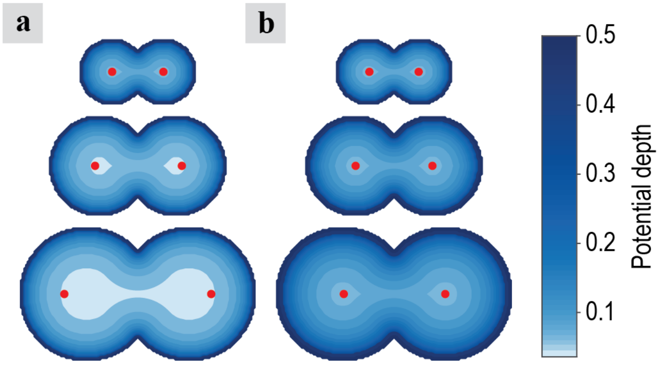


Supplemental Figure 1. Flat-bottomed potentials and scale invariance. **a**, without scale invariance, as the object becomes bigger the potential becomes flat-bottomed, causing the particles to move to the sides. **b**, with scale invariance, the particles have the correct position regardless of scale.

## Supplemental Note 1 Connections to Other Optimization Techniques

Our method of simulation can be thought of as being similar to simulated annealing. Simulated annealing is an optimization method to determine the global ground state of a system. It works by having a prescription of going from one state (set of particle locations) to another state, even if that state has higher in energy. In our case, we get a new state by modeling the particle dynamics and we can reach higher energy (potential energy) states because the particles have momentum. The next important step in simulated annealing is that the temperature of the system is decreased; decreasing the temperature makes it less likely for the system to go from a low energy state to a higher energy state. This is accomplished in our case by damping the particles to remove their momentum.

Our method can also be connected to the gradient descent algorithm with momentum. However, instead of the gradient only depending on some surface $\nabla V$, our gradient also depends on the particle interaction. Additionally, the learning-rate in our method is adaptively set by the Runge-Kutta (2,3) method so that the relative error never increases above some threshold. With this connection to gradient descent, it could be possible to improve the speed of convergence of our method by trying to apply more advanced gradient descent algorithms to our problem, such as Adagrad [1] or Adam [2].

## Supplemental Note 2 Computation of Boundary Curvature

The curvature, $\kappa = (x'y'' - y'x'')/(x'^2 + y'^2)$, is computed by smoothing the boundary by convolution with a Gaussian and then taking the derivatives by convolution with derivatives of a Gaussians. The standard deviation of the Gaussians depends on the object scale, $\lambda$ from (7), $\sigma = \max(1, \text{round}(\lambda/9))$. This value is empirical.

## Supplemental Note 3 Validation Data and Images

The nuclei images used for our experiments were acquired as follows. We cultured squamous cell carcinoma 25 (SCC25) oral cancer cells (epithelial cells from the bottom of the tough) on a coverslip and then fixed them and stained their DNA with 4′,6-diamidino-2-phenylindole (DAPI). The coverlslip was imaged in a fluorescence slide reader with 20x magnification (1 pixel = 0.47 $\mu$m, average nuclei radius 19 pixels). The entire image was segmented using adaptive log-weighted Otsu thresholding [3], which resulted in more than 100,000 objects (either single nuclei or clumps of nuclei). These objects were filtered into five groups according the normalized integrated DAPI intensity (denoted $\langle I_{\text{DAPI}} \rangle$) and the size of each object; examples of the objects from each group can be seen in Supplemental Figure 3. From each group, 484 objects were randomly selected, and the center of each nuclei in all 2,420 objects were manually labeled, resulting in a count of 7,789 nuclei. The red dots in Supplemental Figure 3 are the labeled nuclei centers. As can be seen in Supplemental Figure 3, the nuclei in our data set have a variety of shapes, intensity levels, textures, and noise levels. The nuclei in our data set contain nuclei from each cell phase ($G_1$, S, $G_2$, and M) as well as apoptotic nuclei (dying).

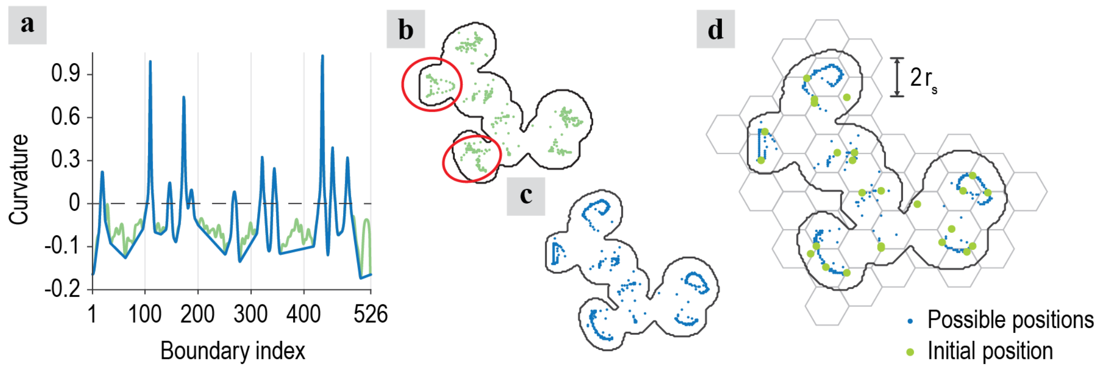


Supplemental Figure 2. Convex hull transformed center of curvature. **a**, curvature (green) and convex hull transformed curvature (blue) versus boundary index. **b**, the set of possible initial particle positions using the curvature data. Note that along the long side of an ellipse the initial points can be far from the geometric center (red circles). **c**, the set of possible initial particle positions using convex hull transformed curvature. **d**, uniform random distribution of the possible initial positions: a hexagonal lattice is overlaid and one possible position from each hexagon is selected.

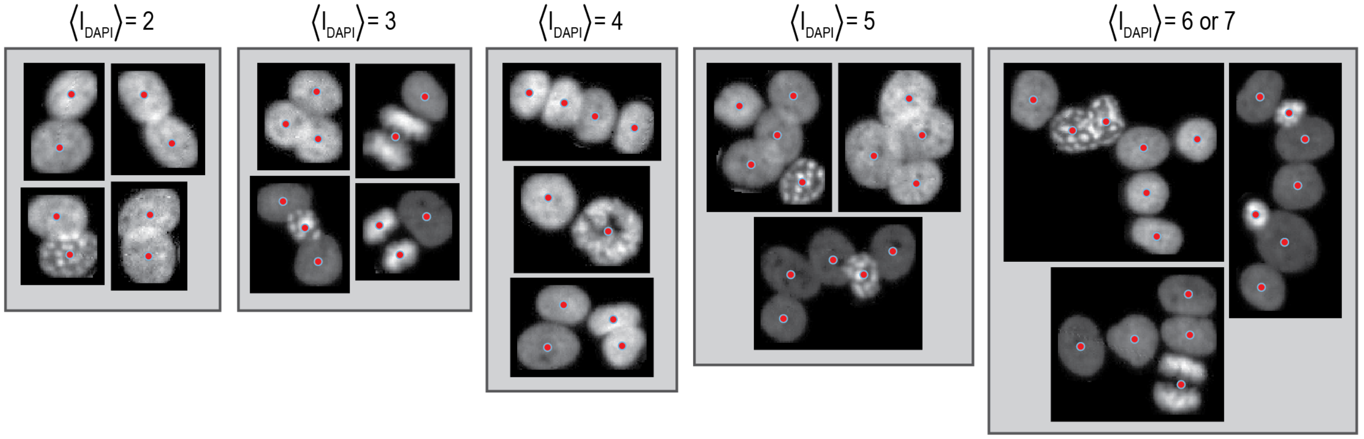


Supplemental Figure 3. Example objects. Each box shows several objects (nuclei clumps) from each of the five groups; the contrast for each object has been enhanced. Labels above the boxes give the normalized integrated DAPI intensity. The red dots represent the labeled nuclei centers, and the edge of the markers represent our expected confidence in their location ($\sim 3$ pixel radius).

## Supplemental Note 4 Locating nuclei centers: previous work and method optimization

A general strategy for locating nuclei centers is searching for circular or elliptical regions in an image. [4] introduced an iterative radial voting approach (also named multi-pass voting, MPV) where cone shaped kernels vote for likely object centers; the cones are initially directed along the image gradient and then in following iterations are directed toward the most likely object centers while decreasing the angular width of the cone. [5] modified this approach to be non-iterative, single-pass voting (SPV) by casting a vote at each image pixel with a large gradient using a cone shaped kernel with an offset Gaussian directed along the image gradient; all of the individual votes are then combined by using a mean-shift clustering algorithm. [6] further modified the SPV approach by first thresholding the image and then only using the boundaries of each object for casting votes along the image gradient.

[7] takes a different approach in using a sliding band filter (SBF) with the image gradient. The SBF works by creating an annular region of fixed width around a given pixel, and then by deforming (sliding) each angular region of the annulus along the radial direction until the dot product between a radial vector field and the image gradient is maximized. This is repeated for every pixel in the image and the resulting voting landscape created from the magnitude of the dot product is used to locate the centers of the nuclei (local maxima). [8] modified this approach to use the image phase congruency instead of the image gradient to address problems when the image contrast is low.

Another popular approach in medical image analysis [9] is Laplacian of Gaussian (LoG) filtering, where the basic principle is to convolute an LoG filter with the image and look for local maxima. [10] introduced a scale normalized LoG filter for selecting the proper LoG scale to use. [11] furthered the method by using a multiscale LoG filter with the maximum scale adaptively limited by the distance transform of the thresholded image. Generalizing these LoG filters for asymmetrical objects, [12] introduced a generalized LoG (gLog) filter where the Gaussian's covariance matrix is not the identity matrix; and, recently, [13] extended this method by creating a set of possible seed-points from each orientation of the gLoG filters and then using mean-shift clustering to combine near by seed-points.

Below we discusses the use and optimization of the seven methods we compared to. The code for these models were received directly from the respective authors or from the code freely available online. The MPV method was used as an ImageJ plugin: https://imagej.nih.gov/ij/plugins/radial-voting.html, and the SBF code was obtained from https://web.fe.up.pt/~quelhas/. The MSER implementation we used was apart of the VLFeat toolbox.

For the MPV, $\mathrm{SPV_{Qi}}$, SBF, and gLoG methods, each of the nuclei images were first contrast enhanced. This contrast enhancement could be called for as our method implicitly corrected for the contrast with the adaptive Otsu thresholding [3]; note that the methods did not perform well, or as well, without the contrast enhancement. The $\mathrm{SPV_{Xu}}$ method, as well as the distance transform, only require the binary mask of each object; so, we directly used the mask from our adaptive log-weighted Otsu thresholding [3] for these methods.

**gLoG optimization:** We optimized over both the small, $\sigma_{\min} \in \{3, 5, 7, 9, 11\}$, and large, $\sigma_{\max} \in \{13, 15, 17, 19, 21, 23\}$, sigma values as well as the mean-shift bandwidth, $b \in r\cdot\{0.3, 0.4, 0.5, 0.6\}$, where $r = 19$ is the average nuclei radius in our images. The parameters that optimized the sum of the $\mathrm{FD}_0$ and $F1_{\delta r=3}$ were $\sigma_{\min} = 9$, $\sigma_{\max} = 15$, and $b = 0.6 \cdot r$. In all the above trials we used 9 orientations of the asymmetric gLoG kernels.

**SBF optimization:** We optimized over the number of angular sections, $N \in \{8, 16, 32\}$, the width of the band, $d \in \{3, 5, 7, 9\}$, and the threshold used to find maxima, $\Theta \in \{0.4, 0.5, 0.6, 0.7, 0.8\}$. We used $r_{\min} = 8$ and $r_{\max} = 30$. The parameters that optimized the sum of the $\mathrm{FD}_0$ and $F1_{\delta r=3}$ were $N = 32$, $d = 5$, and $\Theta = 0.5$.

**$\mathrm{SPV_{Qi}}$ Optimization:** We optimized over the gradient threshold, $\Theta \in \{1, 2.5, 5\}$, the maximum radius, $r_{\max} \in \{34,$

37, 40, 43}, and the bandwidth, $b \in r\cdot\{0.5, 0.6, 0.7, 0.8\}$, where $r = 19$. The minimum radius was set to $r_{\min} = r/3$. We used a radius step size of 3, a cone angle of 60° with angle step size of 3°, and a Gaussian size of $\sigma = 2$. The parameters that optimized the sum of the $\mathrm{FD}_0$ and $F1_{\delta r=3}$ were $\Theta = 2.5$, $r_{\max} = 37$, and $b = 0.7 \cdot r$.

**$\mathrm{SPV}_{\mathrm{Xu}}$ Optimization:** We optimized over the maximum radius, $r_{\max} \in \{21, 24, 27, 30, 33, 36\}$, the ellipticity threshold parameters $e_1 \in \{0.85, 0.875, 0.9, 0.925\}$ and $e_2 \in \{0.025, 0.05, 0.075, 0.1\}$, the Gaussian size $\sigma \in \{3, 6\}$, and the bandwidth, $b \in r\cdot\{0.5, 0.6, 0.7, 0.8\}$, where $r = 19$. The minimum radius was set to $r_{\min} = r/3$. We used a cone angle of 60°. The parameters that optimized the sum of the $\mathrm{FD}_0$ and $F1_{\delta r=3}$ were $r_{\max} = 24$, $e_1 = 0.875$, $e_2 = 0.075$, $\sigma = 6$, and $b = 0.7 \cdot r$.

**MPV Optimization:** As the MPV algorithm was implemented as an imageJ plugin (and not Matlab code), we did not systematically optimize over the parameter values as in the above cases. We used the default threshold on the point selection (1000), and set the average radius to the average radius of our nuclei, 19. The results often contained two seed-points located within $\sim 3$ pixels of each other. Before calculating the results, we first merged each of these double seed-points into a single seed-point.

**MSER:** We tried several parameters for MSER; however, none did very well; therefore, we did not perform systematic optimization.

## Supplemental Note 5 Model parameters

We selected the value of $\lambda_{\max}$ and $r_a$ by evaluating the performance as these parameters are varied, and then selecting the values that maximized the sum of the $F_{1,\,\delta r=3}$ and $\mathrm{FD}_0$ values. Supplemental Figure 4 shows the results of varying these parameters. Note in particular, that as $\lambda_{\max}$ increases to larger values, $F_{1,\,\delta r=3}$ decreases; this is due to the potential becoming flat bottomed as discussed before. See Supplemental Note 6 about scale-invariance for additional discussion about the attractive extent $r_a$.

It is not possible to solve for $A$, $\mu$ and $\sigma$ for all possible values of $d_0$, $r_0$, and $r_a$ in (2). $r_a$ is the most important parameter of these three, and so the primary criterion used in setting $d_0$ and $r_0$ is that the actual location of the potential minimum and attractive extent (when $A$, $\mu$, and $\sigma$ are used to create the potential) are only a few percent away from the values we set. In general, we found $d_0 = -1$ to work until $r_a$ becomes larger than 100, and we found $r_0 \approx 0.15 \cdot r_a$ works well.

The value of $r_s$ was selected after considering its dependence on both the results and the computation time, see Supplemental Note 7 for details.

## Supplemental Note 6 Scale-invariance

Here we explore the issue of scale invariance and flat bottomed potentials. To do this, we scaled the images by a factor and determined our method's performance as the attractive extent $r_a$ is varied. Supplemental Figure 5a,b show the $\mathrm{FD}_0$ value and $F_{1,\,\delta r=3}$ score when scale invariance is not implemented. You can see that as the scale increases, the

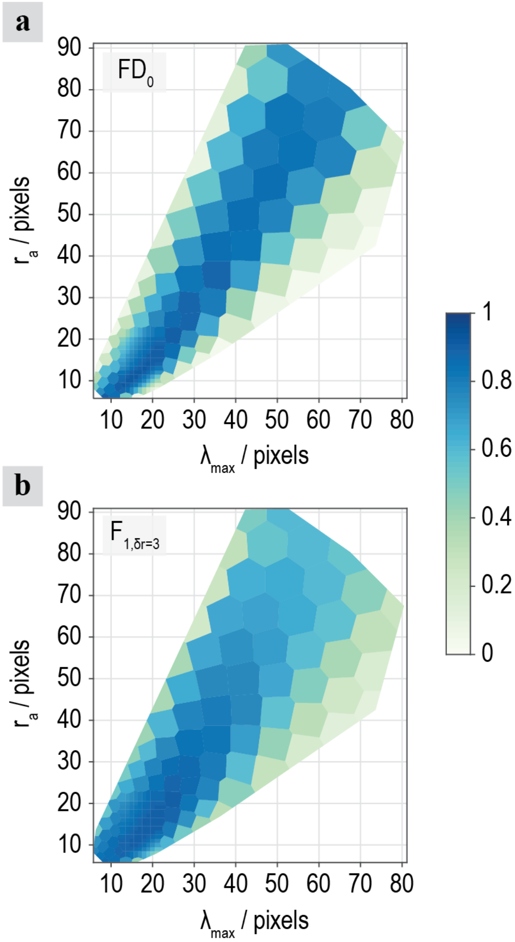


Supplemental Figure 4. **a** and **b** show the $\mathrm{FD}_0$ value and $F_{1,\,\delta r=3}$ score as as $\lambda_{\max}$ and $r_a$ are varied.

attractive extent increases almost linearly. Additionally, as the scale factor increases past $\sim 2$, the $F_1$ score decreases; this is caused by the potential becoming flat bottomed, as in Supplemental Figure 1. Supplemental Figure 5c,d show the results when scale invariance was implemented; you can see that the results are stable at all scale factors.

Supplemental Figure 5 also shows that when the attractive extent is too small or too large that $\mathrm{FD}_0$ and $F_1$ decrease. This is because when $r_a$ is too small, many particle clusters are formed, and when $r_a$ is too large, only a few particle clusters are formed; in both these cases the number of seed points will be wrong which will cause their locations to also be wrong. Remembering that the average nuclei radius in our images is 19 pixels (at scale 1), Supplemental Figure 5a,b show that good results are obtained when the attractive extent is slightly smaller than the average nuclei radius. The same can be seen in Supplemental Figure 5c,d: with the interpretation that $\lambda_{\max}$ is the radius of a nuclei, which is true for an isolated circular nucleus, then the best results are obtained when the attractive extent is $\sim 0.8\lambda_{\max}$.

## Supplemental Note 7 Dependence on particle initialization

We determined the dependence of our method's performance on the initial distribution of particles and the num-

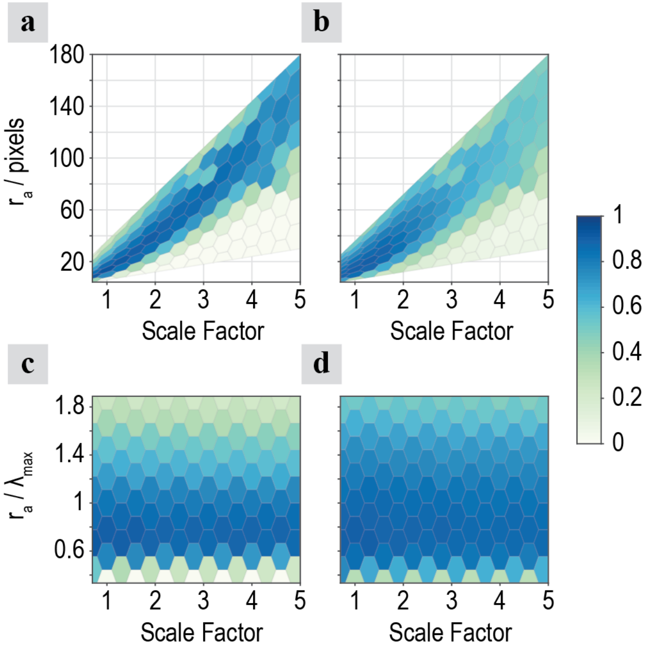


Supplemental Figure 5. **a** shows the $\mathrm{FD}_0$ value and **b** shows and the $F_1$ score at $\delta r = 3$ as the object scale and attractive extent are varied, when scale invariance is not used. **c** and **d** show the same thing when scale invariance is used. In all cases we used $r_0 = \mathrm{round}(0.12\, r_a)$ and $d_0 = \max(0, \log_{10}(r_a/100)) - 1$.

ber of particles. We used four methods of distributing the particles (listed in order of increasing estimated accuracy): random, uniform random, center of curvature (CoC), and convex hull transformed center of curvature (CvxHll CoC). The dependence on the number of particles was determined by using CvxHll CoC point selection method with a Wigner-Seitz radius varying from 2.5 to 20. The results from these trials are shown in Supplemental Figure 6. Supplemental Figure 6a shows that as the density of initial points increases $F_1$ increases, meaning the calculated seed-points get closer to the true points. Supplemental Figure 6c,d show that as the initial particle locations get better, both the $\mathrm{FD}_0$ and $F_1$ values increase. Additionally, Supplemental Figure 6d shows that it is important to have enough initial particles: when $r_s = 20$, $\mathrm{FD}_0$ is low and $\mathrm{FD}_{-1}$ is large because there are not enough particles to detect all of the nuclei centers. Increasing the number of particles with $r_s = 15$ results in a large $\mathrm{FD}_0$ performance boost, and further increase leads to even better performance.

With the results improving with the number of particles, we could use as many particles as possible; however, there is a cost in computation time as the number of particles increases. (This is the reason $r_s = 5$ is our default value even though better results can be obtained with smaller values.) In Supplemental Figure 6b we show the amount of time needed to solve the differential equations per nuclei clump verses the inverse Wigner-Seitz radius. The solver time increases almost linearly with $1/r_s$, with a value of $\sim$ 80 ms at $r_s = 5$, until it finally flattens out. We suspect the time levels off after $r_s = 3$ because all available particles are already selected. Note that the seed-point calculation of each nuclei clump is independent and can be computed in parallel.

## Supplemental Note 8 Requirements of using the distance transform

The distance transform will only work to create a good confining potential if the objects are approximately the same size in each dimension. The reason is as follows: consider a long, thin 2D rectangle oriented so that the long dimension is parallel with the y-axis. The distance transform will only vary along the x-dimension, and therefore the gradient of the distance transform will be zero along the y-axis. This means that there will be no force on the particles along the y-axis pushing the particles to the center. Thus, in general, to be able to use the distance transform, either the objects must naturally be about the same size in each dimension (like 2D nuclei that are not very elliptical), or we must be able to scale the objects to have similar sizes along any direction, which will not be possible in general.

## Supplemental Note 9 Dependence on particle damping rate

In this section we model the particle dynamics in the confining potential of Figure 7c using different particle damping rates, $\alpha$. We modeled the particles 20 times and plot the final cluster positions of each iteration; these results are shown in Supplemental Figure 7. When the damping rate is large, $\alpha = 5 \cdot 10^{-3} t$, the particles are slowed down so quickly that they do not even form clusters, and so there are black dots everywhere. When the damping rate is a bit smaller, $\alpha = 5 \cdot 10^{-4} t$ (the same value used throughout the paper), the particle clusters are more well localized at the correct positions, but there is still some spread and a few points in-between the major clumps. If the damping rate is further decreased to $\alpha = 5 \cdot 10^{-5} t$, then there are no longer any particle clusters in-between the true positions and there is a much smaller spread in the results.

There is a cost to getting the tighter results in computation time. The average solver time for each of the three damping rates is, $91 \pm 30$, $136 \pm 15$, and $421 \pm 44$ ms. Thus, it is faster to simply model the particles $M$ times with $\alpha = 5 \cdot 10^{-4} t$ and then cluster the results of the $M$ simulations (using the same clustering algorithm we use for clustering the particles in the simulation) and keep all clusters that have more than, say, $M/3$ points in them.

## Supplemental Note 10 Available changes and improvements

**Asymmetric particle interaction:** The first possible improvement is related to the particle interaction potential being circularly symmetric. This symmetry can lead to the foci of an ellipse being located instead of the ellipse's geometric center, when several highly elliptical objects are mixed with circular objects with the same area. This problem can be reduced using appropriate initial particle density and initial particle locations; however, a more fundamental fix to the problem has proven difficult. Two potential methods for addressing this issue are as follows: 1) Change the confining potential. Currently, the confining potential will be quite flat

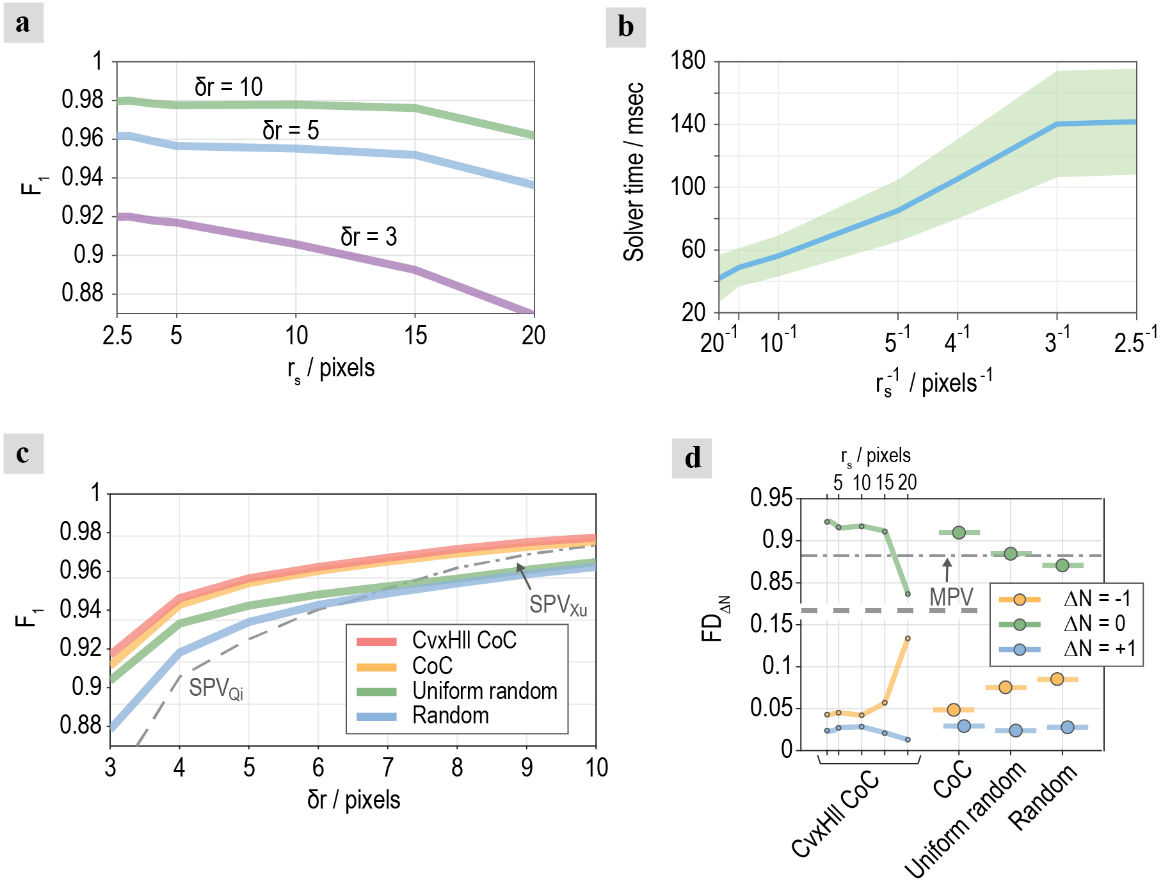


Supplemental Figure 6. **a**, $F_1$ dependence for $\delta r = \{3, 5, 10\}$ of CvxHll CoC particle distribution method versus the density of initial particles. **b**, solver time per nuclei clump (using CvxHll CoC particle distribution method) versus the inverse particle density. Blue line show the average solver time and green shaded region gives $\pm$ one standard deviation. **c**, $F_1$ score versus $\delta r$ for four different initial particle distribution methods. All methods used $r_s = 5$. The dash and dot-dashed lines represent the best values of the methods we compared against in Figure 5. **d**, dependence of $\mathrm{FD}_{\Delta \mathrm{N}}$ on the initial particle distribution method; additionally, the dependence of $\mathrm{FD}_{\Delta \mathrm{N}}$ on the initial particle density using the CvxHll CoC method is shown. The dot-dashed line shows the best $\mathrm{FD}_0$ result of the methods we compared against.

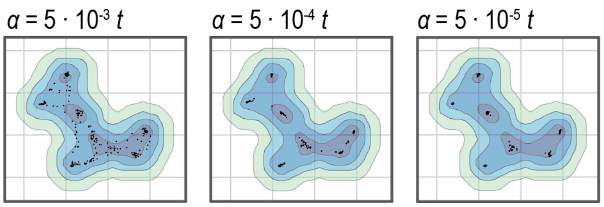


Supplemental Figure 7. The final cluster positions from 20 iterations using three different particle damping rates.

along the major axis of a highly elliptical object because the distance transform only depends on the distance to the nearest boundary pixel; if the potential is modified so that along any line across the object the potential is changing, then the circular symmetry will not be as problematic. 2) Scale the distance between particles using information about the gradient of the confining potential. In the Hamiltonian (1), the argument of the interaction potential could be modified to

$$V_{\mathrm{int}}(|\mathbf{r}_i - \mathbf{r}_j|) \;\rightarrow\; V_{\mathrm{int}}\left(\left|(\mathbf{r}_i - \mathbf{r}_j)\cdot\hat{\mathbf{f}}\left(\nabla V|_{\mathbf{r}_i,\mathbf{r}_j}\right)\right|\right) \qquad (1)$$

where $\hat{\mathbf{f}}(\cdot)$ is a function that takes in the gradient of the confining potential near the particle locations (and potentially along the line connecting the particles) and returns a unit vector that will scale the distance between the particles. In this way, the particle interaction can be made effectively asymmetric and dependent on the local properties of the confining potential. For example, if the confining potential is flat along the line connecting two particles, then with an appropriate choice of $\hat{\mathbf{f}}(\cdot)$ the distance between the particles can be scaled down so that the two particles are attracted to each other.

**Performance metric:** When locating the clusters of scatter point data, previous methods have a metric that can be used to describe how well the data was clustered; for example, k-means can use the average distance to a cluster center and mixture of Gaussians can use the log-likelihood. We currently do not have such a metric for our method, though, we suspect that one possible measure could be related to the final total energy of the particles.

**Clustering:** Our method is able to locate the seed-point of a cluster, but it does not actually divide the scatter point data points into different clusters. One possible method of clustering would be to assign each data point to the nearest

calculated seed-point; potentially better results could be obtained if information from the confining potential is also used.

**Multiple confining potentials:** In regards to biological images, when more than one florescence channel is available, a different confining potential could be created from each. One could then create several different types of particles: particle type 1 would interact with with confining potential 1, particle type 2 would interact with confining potential 2, and so on. Additionally, the particles within each type can have a different interaction potential, and (importantly) particles of different types could interact with each other. This could allow for complex data clustering and pattern recognition to be performed.

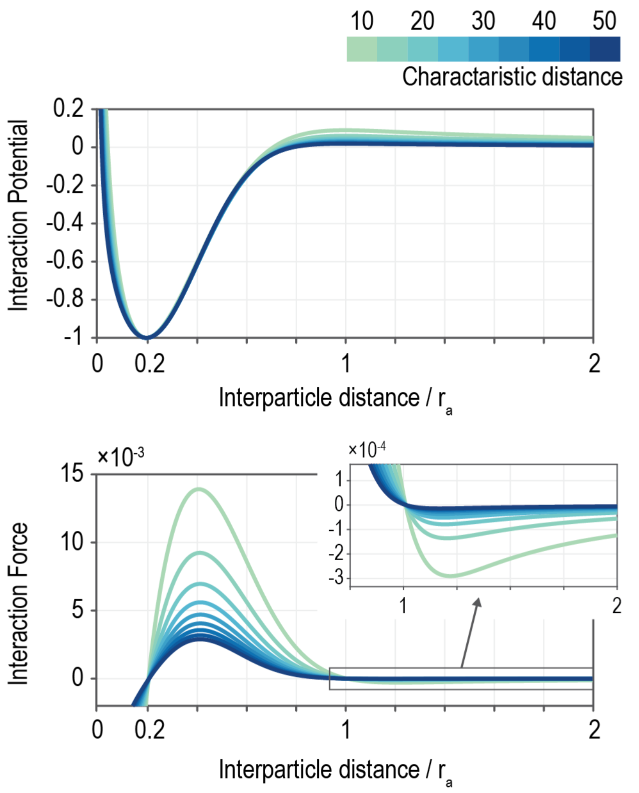


Supplemental Figure 8. The interaction potential and interaction force in data space as the characteristic distance of the solver space is changed. Note, negative force is repulsive and positive force is attractive.

## References


[1] J. Duchi, E. Hazan, and Y. Singer, "Adaptive Subgradient Methods for Online Learning and Stochastic Optimization," *Journal of Machine Learning Research*, vol. 12, pp. 2121–2159, 2011.

[2] D. P. Kingma and J. L. Ba, "Adam: A Method for Stochastic Optimization," *International Conference on Learning Representations 2015*, pp. 1–15, 2015.

[3] N. Otsu, "A threshold selection method from gray-level histograms," *IEEE transactions on systems, man, and cybernetics*, vol. 9, no. 1, pp. 62–66, 1979.

[4] B. Parvin, Q. Yang, J. Han, H. Chang, B. Rydberg, and M. H. Barcellos-Hoff, "Iterative voting for inference of structural saliency and characterization of subcellular events," *IEEE Transactions on Image Processing*, vol. 16, no. 3, pp. 615–623, 2007.

[5] X. Qi, F. Xing, D. J. Foran, and L. Yang, "Robust segmentation of overlapping cells in histopathology specimens using parallel seed detection and repulsive level set," *IEEE Transactions on Biomedical Engineering*, vol. 59, no. 3, pp. 754–765, 2012.

[6] H. Xu, C. Lu, and M. Mandal, "An Efficient Technique for Nuclei Segmentation Based on Ellipse Descriptor Analysis and Improved Seed Detection Algorithm," *IEEE Journal of Biomedical and Health Informatics*, vol. 18, no. 5, pp. 1729–1741, 2014.

[7] P. Quelhas, M. Marcuzzo, A. M. Mendonça, and A. Campilho, "Cell nuclei and cytoplasm joint segmentation using the sliding band filter," *IEEE Transactions on Medical Imaging*, vol. 29, no. 8, pp. 1463–1473, 2010.

[8] T. Esteves, P. Quelhas, A. M. Mendonça, and A. Campilho, "Gradient convergence filters and a phase congruency approach for in vivo cell nuclei detection," *Machine Vision and Applications*, vol. 23, no. 4, pp. 623–638, 2012.

[9] F. Xing and L. Yang, "Robust Nucleus/Cell Detection and Segmentation in Digital Pathology and Microscopy Images: A Comprehensive Review," *IEEE Reviews in Biomedical Engineering*, vol. 3333, no. c, pp. 1–1, 2016.

[10] T. Lindeberg, "Feature Detection with Automatic Scale Selection," *International Journal of Computer Vision*, vol. 30, no. 2, pp. 79 – 116, 1998.

[11] Y. Al-Kofahi, W. Lassoued, W. Lee, and B. Roysam, "Improved automatic detection and segmentation of cell nuclei in histopathology images," *IEEE Transactions on Biomedical Engineering*, vol. 57, no. 4, pp. 841–852, 2010.

[12] H. Kong, H. C. Akakin, and S. E. Sarma, "A generalized laplacian of gaussian filter for blob detection and its applications," *IEEE Transactions on Cybernetics*, vol. 43, no. 6, pp. 1719–1733, 2013.

[13] H. Xu, C. Lu, R. Berendt, N. Jha, M. Mandal, and S. Member, "Automatic Nuclei Detection based on Generalized Laplacian of Gaussian Filters," *Journal of Biomedical and Health Informatics*, vol. XX, no. XX, pp. 1–12, 2016.
